# Supplementary material for: Hund nodal line semimetals: The case of twisted magnetic phase in the double-exchange model
Source: arXiv:1805.03640 ancillary file (2019-01-26)
Supplement: Supplementary file 1 [file supplementary-hund-nodal.pdf]

# Supplementary Material: *Hund nodal line semimetals: The case of twisted magnetic phase in the double-exchange model*

R. Matthias Geilhufe[1], Francisco Guinea[2,3], and Vladimir Juričić[1]
[1]*Nordita, KTH Royal Institute of Technology and Stockholm University, Roslagstullsbacken 23, 10691 Stockholm, Sweden*
[2]*Imdea Nanoscience, Faraday 9, 28015 Madrid, Spain*
[3] *School of Physics and Astronomy. University of Manchester, Manchester M13 9PY*

This Supplementary Material contains: (a) Derivation of the tight binding Hamiltonian in Eq. (4) in the main text; (b) Derivation of a general tight binding Hamiltonian symmetric under the magnetic space group of the spin lattice in twisted magnetic phase; (c) Discussion of the concept of effective time-reversal symmetry; (d) Analysis of the effects of the symmetry breaking perturbations; (e) Calculation of the surface band structure.

## S1. TIGHT-BINDING HAMILTONIAN FOR THE TWISTED MAGNETIC PHASE

To derive the tight binding Hamiltonian we start with four distinct sites within the unit cell (see Fig. 1 in the main text) that exhibit the four spin states $|\pm\phi\rangle$ and $|\pm\phi+\pi\rangle$, given by

$$|\pm\phi\rangle = \frac{1}{\sqrt{2}}\begin{pmatrix}1\\ e^{\pm i\phi}\end{pmatrix}, |\pm\phi+\pi\rangle = \frac{i}{\sqrt{2}}\begin{pmatrix}1\\ -e^{\pm i\phi}\end{pmatrix}. \tag{S1}$$

The hopping amplitude between the sites $i$ and $j$ with the localized spins described in terms of a unit vector $\mathbf{S} = (\cos\phi\sin\theta, \sin\phi\sin\theta, \cos\theta)$ reads

$$\langle\theta_i\phi_i|\theta_j\phi_j\rangle = \cos\frac{\theta_i}{2}\cos\frac{\theta_j}{2} + \sin\frac{\theta_i}{2}\sin\frac{\theta_j}{2}e^{-i(\phi_i-\phi_j)}. \tag{S2}$$

In the basis given by Eq. (S1), the nearest-neighbor hoppings are of the form

$$\begin{aligned} t_{a1b1} &= \langle\phi|\pi-\phi\rangle = \frac{i}{2}(1-e^{-2i\phi}),\ t_{a2b2} = \langle-\phi|\pi+\phi\rangle = \frac{i}{2}(1-e^{2i\phi}),\\ t_{a1a2} &= \langle\phi|-\phi\rangle = \frac{1}{2}(1+e^{-2i\phi}),\ t_{b1b2} = \langle\pi-\phi|\pi+\phi\rangle = \frac{1}{2}(1+e^{2i\phi}), \end{aligned} \tag{S3}$$

and the overall energy scale $t$ is set to unity. Explicitly the form of the tight-binding model given by Eq. (1) in the main text is

$$H_{tw}^{NN} = \sum_{\langle ij\rangle_{\parallel}}(t_{a1b1}a_{1,i}^{\dagger}b_{1,j} + t_{a2b2}a_{2,i}^{\dagger}b_{2,j} + h.c.) + \sum_{\langle ij\rangle_{\perp}}(t_{a1a2}a_{1,i}^{\dagger}a_{2,j} + t_{b1b2}b_{2,i}^{\dagger}b_{1,j} + h.c.), \tag{S4}$$

with $\langle\rangle_{\parallel}$ and $\langle\rangle_{\perp}$ denoting the sum over nearest-neighboring sites in the $x-y$ plane and perpendicular to it, and $\alpha_{s,i}$ is the annihilation operator for an electron at a site $i$ belonging to a sublattice $\alpha = a, b$ in the one of the two inequivalent $x-y$ planes $s = 1, 2$. After Fourier transforming, this Hamiltonian takes the following form in the momentum space

$$\begin{aligned} H_{tw}^{NN} = \sum_{\mathbf{k}}\Big\{&(\cos k_x + \cos k_y)\left[i\left(1-e^{-2i\phi}\right)a_{1,\mathbf{k}}^{\dagger}b_{1,\mathbf{k}} + i\left(1-e^{2i\phi}\right)a_{2,\mathbf{k}}^{\dagger}b_{2,\mathbf{k}}\right]\\ &+\cos k_z \times \left[\left(1+e^{-2i\phi}\right)a_{1,\mathbf{k}}^{\dagger}a_{2,\mathbf{k}} + \left(1+e^{2i\phi}\right)b_{1,\mathbf{k}}^{\dagger}b_{2,\mathbf{k}}\right] + h.c.\Big\}, \end{aligned} \tag{S5}$$

with the lattice spacing of the original cubic lattice set to unity, $a = 1$. This Hamiltonian can then be readily rewritten in terms of the Pauli matrices acting in the basis $\psi_{\mathbf{k}} = (a_{1,\mathbf{k}}, b_{1,\mathbf{k}}, a_{2,\mathbf{k}}, b_{2,\mathbf{k}})^{\intercal}$, yielding Eq. (4) in the main text.

## S2. TIGHT BINDING HAMILTONIAN CONSTRAINED BY THE LATTICE SYMMETRIES

We now construct a general lattice tight binding Hamiltonian in the twisted phase (1) consistent with the symmetries discussed above. The form of the Hamiltonian in the momentum space is

$$H(\mathbf{k},\phi) = \sum_{\mu\nu} f_{\mu\nu}(\mathbf{k})F_{\mu\nu}(\phi)\sigma_{\mu}\otimes\tau_{\nu}, \tag{S6}$$

| $\sigma_\mu$ \ $\tau_\nu$ | 0 | 1 | 2 | 3 |
|---|---|---|---|---|
| 0 | + + | - - | - + | - - |
| 1 | - + | + - | + + | + - |
| 2 | + - | - + | - - | - + |
| 3 | + - | - + | - - | - + |

TABLE S1. Commutation (+) and anticommutation (-) of $\sigma_\mu \otimes \tau_\nu$ with respect to the antiunitary operation $\{\mathrm{KIC}_{2z}|\frac{1}{2},-\frac{1}{2},\frac{1}{2}\} = -i\sigma_3 \otimes \tau_2 \hat{K}$ (black) and the unitary operation $\{\mathrm{IC}_{2z}|\frac{1}{2},-\frac{1}{2},0\} = i\sigma_1 \otimes \tau_2$ (red).

with $\mu, \nu = 0,1,2,3$.

First, consider non-symmorphic unitary operation $\mathrm{IC}_{2z}$, which constraints the above Hamiltonian as

$$H(k_\perp, k_z, \phi) = (i\sigma_1 \otimes \tau_2)^\dagger H(k_\perp, -k_z, \phi) i\sigma_1 \otimes \tau_2, \tag{S7}$$

since under this transformation $(k_\perp, k_z) \to (k_\perp, -k_z)$, and $k_\perp \equiv (k_+, k_-)$. Second, the invariance of the Hamiltonian under non-symmorphic antiunitary operation $\mathrm{KIC}_{2z}$ yields the following condition

$$H(k_\perp, k_z, \phi) = -(-i\sigma_3 \otimes \tau_2)^\dagger H(-k_\perp, k_z, \phi)^* (-i\sigma_3 \otimes \tau_2), \tag{S8}$$

since under this operation momentum transforms as $(k_\perp, k_z) \to (-k_\perp, k_z)$, and the additional minus sign arises from the fact that this operation involves an odd number of partial translations, as opposed to $\mathrm{IC}_{2z}$ with two half-translations.

Moreover, Hamiltonian has to be invariant under the mirror symmetry through the $z=0$ plane accompanied by $\phi \to -\phi$, which is represented by the matrix $\sigma_1 \otimes \tau_0$,

$$H(k_\perp, k_z, \phi) = (\sigma_1 \otimes \tau_0)^\dagger H(k_\perp, -k_z, -\phi) \sigma_1 \otimes \tau_0, \tag{S9}$$

This operation lifts the degeneracy between even and odd functions $F_{\mu\nu}(\phi)$ of the angle $\phi$ appearing in the general Hamiltonian given by Eq. (S6).

These three symmetry operations combined, using transformation properties of the Pauli matrices in Table S1, yield the following form of the general Hamiltonian

$$H(\mathbf{k}, \phi) = \sum_{j=1}^{4} H^{(j)}(\mathbf{k}, \phi), \tag{S10}$$

with

$$H^{(j)}(\mathbf{k}, \phi) = \sum_{\alpha=e,o} \sum_{\mu\nu} f^{(j)}_{\mu\nu}(\mathbf{k}) F^{j,\alpha}_{\mu\nu}(\phi) \Sigma^{j,\alpha}_{\mu\nu}. \tag{S11}$$

Here, $F^{j,e,o}_{\mu\nu}(\phi)$ are respectively even and odd functions of $\phi$, $F^{j,e,o}_{\mu\nu}(\phi) = \pm F^{j,e,o}_{\mu\nu}(-\phi)$, and index $j$ labels the four combinations of the parities of the function $f^{(j)}$ under the change of sign of the $x-y$ (in-plane) and the $z$ components of the momentum, which appear due to the form of the symmetry transformations given by Eqs. (S7) and (S8). The form of the matrices appearing in the Hamiltonian is given in the Table S2.

It is worthwhile noticing that the nearest-neighbor Hamiltonian in Eq. (4) in the main text, realizes the case with $j=1$, see also Table S2. Namely, the corresponding functions of the momentum are even under both momentum exchange operations, and symmetry allowed matrices off-diagonal in only one of the subspaces ($1,2$ or $a,b$) appear in the Hamiltonian in Eq. (5) since the lattice Hamiltonian involves only nearest-neighbor hopping.

## S3. THE CONCEPT OF EFFECTIVE TIME-REVERSAL SYMMETRY

The time reversal symmetry is an antiunitary symmetry and can be treated in the framework of the Shubnikov group construction[1,2]. For a time reversal symmetric system, the symmetry group is given by the Suhbnikov group of the second kind, or gray group,

$$\mathcal{G}^{II} = \mathcal{G} + T\mathcal{G}. \tag{S12}$$

| j | $f^{(j)}_{\mu\nu}(k_\perp, k_z)$ | $\Sigma^{j,e}_{\mu\nu}$ | $\Sigma^{j,o}_{\mu\nu}$ |
|---|---|---|---|
| 1 | + + | $\sigma_0 \otimes \tau_2,\ \sigma_1 \otimes \tau_0$ | $\sigma_2 \otimes \tau_1,\ \sigma_2 \otimes \tau_3,\ \sigma_3 \otimes \tau_3$ |
| 2 | + - | $\sigma_2 \otimes \tau_2,\ \sigma_3 \otimes \tau_2$ | $\sigma_0 \otimes \tau_1,\ \sigma_0 \otimes \tau_3$ |
| 3 | - + | $\sigma_0 \otimes \tau_0,\ \sigma_1 \otimes \tau_2$ | |
| 4 | - - | $\sigma_2 \otimes \tau_0, \sigma_3 \otimes \tau_0$ | $\sigma_1 \otimes \tau_1,\ \sigma_1 \otimes \tau_3$ |

TABLE S2. Elements of the symmetry constrained Hamiltonian in Eq. (S10). First column: Parity of the function $f^{(j)}_{\mu\nu}(k_\perp, k_z)$ under $k_\perp \to -k_\perp$ (black) and $k_z \to -k_z$ (red), with $k_\perp \equiv (k_+, k_-)$. Second and third columns: Symmetry allowed matrices $\Sigma^{j;\alpha}_{\mu\nu}$, with $\alpha = e, o$ multiplying the corresponding functions $f^{(j)}(\mathbf{k})$ in the Hamiltonian in Eq. (S10).

Considering systems where time-reversal symmetry is broken, but combinations of symmetry elements $g$ with time-reversal $T$ are global symmetries $gT$, the resulting symmetry group is the Suhbnikov group of the third kind

$$\mathcal{G}^{III} = \mathcal{N} + T\left(\mathcal{G} - \mathcal{N}\right), \tag{S13}$$

where $\mathcal{N} \subset \mathcal{G}$ denotes a normal divisor of $\mathcal{G}$ of index 2. For fermionic systems, time-reversal squares to minus one, i.e., $T^2 = -1$. The framework is generalized if an antiunitary symmetry $A$ is present, which has the same algebraic property, i.e., $A^2 = -1$,

$$\mathcal{G}^{II} = \mathcal{G} + A\mathcal{G}, \qquad \mathcal{G}^{III} = \mathcal{N} + A\left(\mathcal{G} - \mathcal{N}\right). \tag{S14}$$

For example, such an *effective time-reversal symmetry* was discussed in Ref. 3, in the form of a nonsymmorphic antiferromagnetic time-reversal $\tilde{T} = (T, \mathbf{t})$, with $\mathbf{t}$ being a fractional lattice translation. In the present paper, such an effective time-reversal symmetry is constructed as a combination of a mirror symmetry with a fractional lattice translation and complex conjugation, $\{\mathrm{KIC}_{2z}|1/2, -1/2, 1/2\}$, see also Table I in the main text.

## S4. ANALYSIS OF THE EFFECTS OF SYMMETRY BREAKING PERTURBATIONS

In the twisted phase the localized spins are aligned in plane as described by Eq. (2) and shown in Fig. 1 in the main text. The fourfold degenerate line node at the edges of the $k_z = \pm\pi/2$ planes are protected by a combination of $\mathrm{IC_{2z}}$ and $\mathrm{KIC_{2z}}$. In the following, we consider alternations in the spin structure of the material, which can break these symmetries. First, we introduce a slight tilt of the magnetic moments by an angle $\theta$ in $z$-direction with a staggering between the two layers in the unit cell. The resulting localized spins read

$$\mathbf{S}_i = \cos\phi \sin\theta(-1)^{x+y}\mathbf{e}_x + \sin\phi\sin\theta(-1)^z\mathbf{e}_y + \cos\theta(-1)^z\mathbf{e}_z. \tag{S15}$$

Consequently, $\mathrm{IC_{2z}}$ and K symmetries of the system are broken, while the $\mathrm{KIC_{2z}}$ symmetry is kept intact. This spin configuration, using the form of the tight-binding Hamiltonian in the double exchange model, Eq. (1) in the main text, yields a perturbation of the form,

$$V_{\mathrm{KIC2}} = -\left(\cos k_x + \cos k_y\right) \times \left[\frac{\cot\theta}{\sin\theta}\,\sigma_3 \otimes \tau_2 + \cot^2\theta\,\sigma_0 \otimes \tau_2\right]. \tag{S16}$$

Notice that $V_{\mathrm{KIC2}}$ vanishes for $\theta = \pi/2$, which represents the twisted phase. For small derivations $\theta = \pi/2 + \delta$,

$$V_{\mathrm{KIC2}} \approx -\delta\left(\cos k_x + \cos k_y\right)\sigma_3 \otimes \tau_2. \tag{S17}$$

$V_{\mathrm{KIC2}}$ vanishes on the BZ boundary plane $k_x \pm k_y = \pm\pi$, and consequently preserves the degeneracy of the line node, as shown in Fig. 3a in the main text. Otherwise, it splits the twofold degeneracy of the bands in the $k_z = 0$ and $k_z = \pi/2$ planes, since it breaks $\mathrm{IC_{2z}}$ symmetry. Furthermore, the symmetry $\mathrm{KIC_{2z}}$ allows for a perturbation of the form

$$V_{\mathrm{KIC2}} \approx -\delta\left(\cos\frac{k_x}{2} + \cos\frac{k_y}{2}\right)\sigma_3 \otimes \tau_2, \tag{S18}$$

which also breaks both $\mathrm{IC_{2z}}$ and K symmetries but in contrast gives rise to a mass term which is non-vanishing along the edge of the BZ boundary at $k_z = \pi/2$. The nodal line is then gapped, but the Kramers degeneracy is preserved, leading to two pairs of nodal lines symmetrically split about the zero energy, as shown in Fig. 3b in the main text.

We now consider slightly twisted spins in $z$-direction that in addition stagger between $a$- and $b$-sites, with the form

$$\mathbf{S}_i = \cos\phi\sin\theta(-1)^{x+y}\mathbf{e}_x + \sin\phi\sin\theta(-1)^{z}\mathbf{e}_y + \cos\theta(-1)^{x+y}\mathbf{e}_z. \tag{S19}$$

For this perturbation, the $\mathrm{IC_{2z}}$ and $\mathrm{KIC2_2}$ symmetries are broken and only the K symmetry is kept. The resulting perturbation reads

$$V_{\mathrm{K}} = \cos\frac{k_z}{2}\left[\frac{\cot\theta}{\sin\theta}\,\sigma_1\otimes\tau_3 + \cot^2\theta\,\sigma_1\otimes\tau_0\right]. \tag{S20}$$

For very small deviations from the twisted phase we obtain

$$V_{\mathrm{K}} \approx \delta\,\cos\frac{k_z}{2}\,\sigma_1\otimes\tau_3. \tag{S21}$$

Similarly to $V_{\mathrm{KIC2}}$, $V_{\mathrm{K}}$ leads to a fully gapped band structure (Fig. 3b in the main text).

## S5. CALCULATION OF THE SURFACE BAND STRUCTURE

To calculate the surface electronic structure, we have considered a tight-binding model which is periodic in the $k_x$ and $k_y$ direction, containing 151 layers along the crystallographic $z$ direction. The angle $\phi$ of the twisted phase was chosen similarly as before, i.e., $\phi = 1$.

The model itself is constructed via the partial Fourier transform of the Hamiltonian in Eq. (S4) along the $x_+$ and $x_-$ directions, while keeping the $z$ direction open, i.e. translational symmetry is broken in this direction. Within each layer $n$ in $z$-direction, the wave function $\psi_{\mathbf{k}}^{(n)}$ has the components $\psi_{\mathbf{k}}^{(n)} = (a_{1,\mathbf{k}}^{(n)}, b_{1,\mathbf{k}}^{(n)}, a_{2,\mathbf{k}}^{(n)}, b_{2,\mathbf{k}}^{(n)})^{\intercal}$, where $\mathbf{k} = (k_x, k_y)$. The total Hamiltonian is the constructed similarly as in Ref. 4, via

$$H = \sum_{n=1}^{N} \psi_{\mathbf{k}}^{(n)\,\dagger}\left(T\psi_{\mathbf{k}}^{(n-1)} + M\psi_{\mathbf{k}}^{(n)} + T^{\dagger}\psi_{\mathbf{k}}^{(n+1)}\right), \tag{S22}$$

where we have imposed the boundary conditions $\psi_{\mathbf{k}}^{(0)} = \psi_{\mathbf{k}}^{(N+1)} = 0$. The corresponding hopping matrices are given by

$$M = (\cos k_x + \cos k_y)\left[-(1-\cos 2\phi)\sigma_0\otimes\tau_2 - \sin 2\phi\,\sigma_3\otimes\tau_1\right] + \left[(1+\cos 2\phi)\sigma_1\otimes\tau_0 + \sin 2\phi\,\sigma_2\otimes\tau_3\right], \tag{S23}$$

and

$$T = \frac{1}{2}\left[(1+\cos 2\phi)\,\sigma_1\otimes\tau_0 + i\sin 2\phi\,\sigma_1\otimes\tau_3 - i(1+\cos 2\phi)\,\sigma_2\otimes\tau_0 + \sin 2\phi\,\sigma_2\otimes\tau_3\right]. \tag{S24}$$

We calculate the Green function of the system from the inverse of the Hamiltonian, via $G(\mathbf{k}, E) = [H(\mathbf{k}) - (E + i\delta)]^{-1}$. The corresponding Bloch spectral function is calculated via

$$A(\mathbf{k}, E) = \frac{1}{\pi}\,\mathrm{Im}\,\mathrm{Tr}\,G(\mathbf{k}, E), \tag{S25}$$

and exhibits poles when $E$ crosses a band for $\delta = 0$. To obtain information about the surface layer we investigate the surface contribution of $G$ within the first and the $Nth$ layer.


[1] C. Bradley and A. Cracknell, *The mathematical theory of symmetry in solids: representation theory for point groups and space groups* (Oxford University Press, 2010).

[2] W. Hergert and R. M. Geilhufe, *Group Theory in Solid State Physics and Photonics: Problem Solving with Mathematica* (John Wiley & Sons, 2018).

[3] S. M. Young and B. J. Wieder, Phys. Rev. Lett. **118**, 186401 (2017).

[4] M. Biderang, A. Leonhardt, N. Raghuvanshi, A. P. Schnyder, and A. Akbari, arXiv preprint arXiv:1802.09139 (2018).
